# Supplementary material for: Designing Informative Rating Systems: Evidence from an Online Labor Market
Source: arXiv:1810.13028 source file (2019-07-22)
Supplement: Supplementary file 1 [file online_supplement.tex]

\documentclass[msom,blindrev]{informs3} % current default for manuscript submission
%\documentclass[msom,nonblindrev]{informs3}

%%\OneAndAHalfSpacedXI
\OneAndAHalfSpacedXII % Current default line spacing
%%\DoubleSpacedXII
%\DoubleSpacedXI

% If hyperref is used, dvi-to-ps driver of choice must be declared as
%   an additional option to the \documentclass. For example
%\documentclass[dvips,msom]{informs3}      % if dvips is used
%\documentclass[dvipsone,msom]{informs3}   % if dvipsone is used, etc.
% Private macros here (check that there is no clash with the style)

% Natbib setup for author-year style
\usepackage{natbib}
\bibpunct[, ]{(}{)}{,}{a}{}{,}%
%
%
%
%
%

%% Setup of theorem styles. Outcomment only one.
%% Preferred default is the first option.
\TheoremsNumberedThrough     % Preferred (Theorem 1, Lemma 1, Theorem 2)
%\TheoremsNumberedByChapter  % (Theorem 1.1, Lema 1.1, Theorem 1.2)

%% Setup of the equation numbering system. Outcomment only one.
%% Preferred default is the first option.
\EquationsNumberedThrough    % Default: (1), (2), ...
%\EquationsNumberedBySection % (1.1), (1.2), ...

% In the reviewing and copyediting stage enter the manuscript number.
%\MANUSCRIPTNO{} % When the article is logged in and DOI assigned to it,
%   this manuscript number is no longer necessary

%\usepackage{setspace}

\usepackage{thmtools}
\usepackage{thm-restate}
\usepackage{booktabs} % For formal tables
\usepackage{tabularx}
\usepackage{amsmath, xr}
\usepackage{xcolor}
\usepackage{bibentry}
\usepackage[hidelinks]{hyperref}

\usepackage{float,subcaption,placeins}
%\usepackage[demo]{graphicx}

%\externaldocument{online_supplement}
% \newtheorem{assumption}[theorem]{Assumption}
% \newtheorem{remark}[theorem]{Remark}

% \newcommand{\Halmos}{$\square$}
%\newcommand{\proof}[0]{\begin{proof}}

 % Real numbers
 % Real numbers
 % Integers
 % Expectation

	%% Title portion. Note the short title for running heads 
	\title{Online supplement for -- Designing Informative Rating Systems: Evidence from an Online Labor Market}  
	
	\date{}
	
	%\author{Nikhil Garg}
	%\affiliation{%
	%	\institution{Stanford University}
	%	\department{Department of Electrical Engineering}
	%}
	%\email{nkgarg@stanford.edu}
	%\author{Ramesh Johari}
	%\affiliation{%
	%	\institution{Stanford University}
	%	\department{Department of Management Science \& Engineering}
	%}
	%\email{rjohari@stanford.edu}
	%\begin{abstract}
	%\input{abstract.tex}
	%\end{abstract}
	%
	
%	\newcommand{\todo}[1]{\noindent{\textcolor{green}{\textbf{TODO}: \textsf{#1}}}}

	\externaldocument{draft_MSOM}
		\SingleSpacedXI
	\begin{document}
%	\maketitle
	
%	\input{appendix_labor_onlinesupplement.tex}
%	\input{appendix_mturk_onlinesupplement.tex}
%	\input{appendix_theory.tex}
	%\input{binarymodel.tex}
	%\input{appendix_theory.tex}

	%\newpage
	%\pagebreak
%	\newpage
%	\pagebreak
%	\FloatBarrier
%	\appendix
	
	 \begin{APPENDICES}
		\input{appendix_labor.tex}
		\input{app_mturk_new.tex}
		\input{mturk.tex}
		\input{appendix_mturk.tex}
		\input{appendix_theory.tex}
	\end{APPENDICES}
	\bibliographystyle{informs2014}
\nobibliography{bib}	
\end{document}
